# Supplementary material for: Low-Rate Overuse Flow Tracer (LOFT): An Efficient and Scalable Algorithm for Detecting Overuse Flows
Source: arXiv:2102.01397 source file (2021-02-02)
Supplement: Supplementary file 1 [file appendix.tex]

For parts of our evaluation we rely on a CAIDA dataset of captured network
traffic~\cite{caida201810}, which we aggregate into flows.
Figure~\ref{fig:graph_caida_dist} shows the distribution of flow sizes in this
dataset.

\begin{figure}[th]
    \centering \includegraphics[width=\columnwidth]{fig/graph_caida_dist} \caption{The
    cumulative distribution of flow sizes in the CAIDA
    traffic.}  \label{fig:graph_caida_dist}
\end{figure}
